# Supplementary material for: Large-Signal Stability Guarantees for Cycle-by-Cycle Controlled DC-DC Converters
Source: arXiv:2205.10155 source file (2022-10-16)
Supplement: Supplementary file 1 [file 7_appendix.tex]

%\section{Appendix}
% \begin{appendices}
% % \section{Continuity Theorem for Low-pass Filter} \label{sec:proof_filter_cont}
% % \subsection{Continuity Theorem for General Linear Filter}
% % The current control loop with filter can be modeled as
% % \begin{align}
% %      \label{eqn:cc_filter_1x} i_p[n] =& \,i_p[n-1] -m_2t_{\text{off}} +m_1\,t_{\text{on}}[n],\\
% %       i_c [n] =& \, q(t)\bigg\rvert_{t=t_{\text{on}}[n]}q(T_{\text{off}}) i_c[n-1] \nonumber \\
% %      \label{eqn:cc_filter_2} &+ \left(i_m(t) u(t) * h(t)\right)\bigg\rvert_{t=t_{\text{on}}[n]}
% % \end{align}
% % where
% % \begin{align}
% %     i_m(t) = i_p[n-1] - m_2T_{\text{off}} + m_1 t + w(t).
% % \end{align}
% % the desired current $I_c$ and actual current $I_p$ at the equilibrium, satisfies
% % \begin{align} \label{eqn:equic}
% %     I_c = \frac{\left(\left( I_p -m_2T_{\text{off}} + m_1 \, t + w(t) \right) u(t)*h(t)\right)\bigg\vert_{t=T_{\text{on}}}
% %     }{1-q(T_{\text{on}})q(T_{\text{off}})}.
% % \end{align}
% % From Theorem \ref{th:equexcond}, the continuous static mapping is equivalent to the monotonic current sensor output. Therefore, the continuity condition can be equivalently expressed as
% % \begin{align} \label{eqn:cont_filter}
% %     & (I_p-m_1T_{\text{off}})\left( u(t) * h(t)\right)^{'} 
% %      + 
% %     I_cq^{'}(t)q(T_{\text{off}}) \nonumber \\
% %     & +
% %     \left((m_1t+w(t))u(t)*h(t)\right)^{'}
% %     >0,
% % \end{align}
% % for all $t > 0^{+}$.
% % For all $t>0^{+}$, $u(t)*h(t)$ and $m_1t\,u(t)*h(t)$ are differentiable
% % \begin{align}
% %      \label{eqn:conv_eq1} \left( m_1t\, u(t)*h(t) \right)^{'} &=  m_1u(t)*h(t) \\
% %      \label{eqn:conv_eq2} \left( u(t)*h(t) \right)^{'} &=  h(t)
% % \end{align}
% % The zero state response of the filter given input signal $w(t)u(t)$ is
% % \begin{align}  \label{eqn:fu_conv_h}
% %     w(t)u(t)*h(t) = \left(w(t)*h(t) - \frac{g(0)}{q(0)} q(t)\right)u(t).
% % \end{align}
% % where $\left(w(t)*h(t)\right) u(t)$ is the forced response and rest is natural response.
% % We denote the forced response as $g(t) \triangleq w(t)*h(t)$.
% % For all $t>0^{+}$, $w(t)u(t)*h(t)$ is differentiable
% % \begin{align} \label{eqn:conv_eq_new} 
% %     \left(w(t) u(t)*h(t)\right)^{'} = g'(t) u(t)- \frac{g(0)}{q(0)}q'(t) u(t)
% % \end{align}
% % Therefore, the continuity condition can be equivalently expressed as 
% % \begin{align}
% %     m_1u(t)*h(t) + g'(t) u(t)- \frac{g(0)}{q(0)}q'(t) u(t) > 0
% % \end{align}
% % \subsection{Continuity Theorem for First-Order Low-Pass Filter}
% % For a first-order low-pass filter with time constant $\tau$, the impulse response $h(t)$ and zero input response $q(t)$
% % \begin{align} \label{eqn:ht_def}
% %     h(t) = \frac{e^{-\frac{t}{\tau}}}{\tau}\,u(t) \quad q(t) = e^{-\frac{t}{\tau}}\,u(t).
% % \end{align}
% % The frequency response function of the filter is
% % \begin{align} \label{eqn:hjw}
% %     H(j\omega) = \frac{1}{1+j\omega\tau}.
% % \end{align}
% % Substitute (\ref{eqn:ht_def}) and (\ref{eqn:hjw}) into (\ref{eqn:conv_eq_new}),
% % \begin{align}
% %     g'(t) = & \int_{-\infty}^{+\infty} j\omega W(\omega) H(\omega) e^{j\omega t}\,d\omega
% %     \nonumber
% % \end{align}
% % \begin{align}
% %     = & \int_{0}^{+\infty} \frac{e^{j\frac{\pi}{2}} |\omega| W(\omega)}{\sqrt{1+\omega^2\tau^2}}  e^{ -j(\frac{\pi}{2} -\delta)} e^{j\omega t}\,d\omega \nonumber \\ 
% %     & + \int_{-\infty}^{0} \frac{e^{-j\frac{\pi}{2}}|\omega| W(\omega)}{\sqrt{1+\omega^2\tau^2}}  e^{j (\frac{\pi}{2}-\delta)} e^{j\omega t}\,d \omega \nonumber
% % \end{align}
% % \begin{align}
% %     = & \int_{0}^{+\infty} \frac{ |\omega| W(\omega)}{\sqrt{1+\omega^2\tau^2}} e^{ j\delta} e^{j\omega t}\,d\omega \nonumber \\
% %     & + \int_{-\infty}^{0} \frac{|\omega| W(\omega)}{\sqrt{1+\omega^2\tau^2}}  e^{-j\delta} e^{j\omega t}\,d\omega,
% % \end{align}
% % where $\delta = \text{tan}^{-1}(1/(\omega \tau))$.\\
% % By assumption that $\omega\tau \gg 1$, 
% % \begin{align} \label{eqn:g_pr_t}
% %     g'(t) & \approx \int_{0}^{+\infty} \frac{  W(\omega)}{\tau} e^{ j\delta} e^{j\omega t}\,d\omega + \int_{-\infty}^{0} \frac{W(\omega)}{\tau}  e^{-j\delta} e^{j\omega t}\,d\omega \nonumber \\  
% %     & \approx \frac{1}{\tau}\int_{-\infty}^{+\infty} W(\omega) e^{j\omega t}\,d\omega = \frac{w(t)}{\tau}.
% % \end{align}
% % \begin{align} \label{eqn:g_zero_t}
% %  g(0) = & \int_{-\infty}^{+\infty} W(\omega) H(\omega) e^{j\omega t}\,d\omega \bigg \rvert_{t = 0} = \int_{-\infty}^{+\infty} W(\omega) H(\omega)\,d\omega \nonumber\\
% %  & \approx \int_{-\infty}^{+\infty} \frac{W(\omega)}{j\omega}\,d\omega 
% % \end{align}
% % \begin{align}
% %     g(t) = & \int_{-\infty}^{+\infty} W(\omega) H(\omega) e^{j\omega t}\,d\omega \nonumber \\
% %     = & 2 \text{Re} \left[\int_{0}^{+\infty} \frac{W(\omega)}{\sqrt{1+\omega^2\tau^2}} e^{ -j(\frac{\pi}{2} -\delta)} e^{j\omega t}\,d\omega \right]
% % \end{align}
% % \begin{align}\label{eqn:s_lower_bound1_simp2}
% %     |g(t)| < & \int_{-\infty}^{+\infty} |W(\omega)||H(\omega)| e^{j\omega t}\,d\omega = \int_{-\infty}^{+\infty} \frac{|W(\omega)|}{\sqrt{1 + \omega^2\tau^2}} \,d\omega \nonumber \\
% %     < & \frac{1}{\omega_{l}\tau} \int_{-\infty}^{+\infty} |W(\omega)| \,d\omega < \frac{A}{\omega_l \tau}.
% % \end{align}
% % We substitute (\ref{eqn:ht_def}), (\ref{eqn:g_pr_t}) and (\ref{eqn:g_zero_t}) into the (\ref{eqn:conv_eq_new}) 
% % \begin{align}
% %     \left(w(t) u(t)*h(t)\right)^{'} = \frac{w(t)}{\tau} + \frac{e^{-\frac{t}{\tau}}}{\tau}\int_{-\infty}^{+\infty} \frac{W(\omega)}{j\omega}\,d\omega 
% % \end{align}
% % Therefore, 
% % \begin{align}
% %     \bigg| \int_{-\infty}^{+\infty} \frac{W(\omega)}{j\omega}\,d\omega \bigg| =|g(0)|< \frac{A_{ub}}{\omega_l \tau}
% % \end{align}
% % In worst-case $I_p = m_1T_{\text{off}}$, (\ref{eqn:cont_filter}) can be bounded from below by
% % \begin{align} \label{eqn:bd_slope}
% %      & q^{'}(t)q(T_{\text{off}})I_c
% %     + \left((m_1t+w(t))u(t)*h(t)\right)^{'}\nonumber \\
% %     = & -\frac{e^{-\frac{t}{\tau}}}{\tau}q(T_{\text{off}})I_c + m_1(1-e^{-\frac{t}{\tau}}) + \frac{w(t)}{\tau} \nonumber \\
% %     & + \frac{e^{-\frac{t}{\tau}}}{\tau}\int_{-\infty}^{+\infty} \frac{W(\omega)}{j\omega}\,d\omega \nonumber \\
% %     \ge & - q(T_{\text{max}})I_{\text{max}} - \frac{A_{ub}}{\tau} - \frac{1}{\omega_l \tau} \frac{A_{ub}}{\tau}
% % \end{align}
% % We notice if we only require $t>0$,  (\ref{eqn:bd_slope}) may be neg
% \section{Linearized Model of the Current-Control Loop with Low-Pass Filter} \label{sec:proofoptsc}
% % We observe that both $a_{\text{min}}$ and  $a_{\text{max}}$ are right-shifted with increasing $m_s$. Therefore the optimal $m_s$ should make $a_{\text{min}} = -a_{\text{max}}$ for shortest settling time in the worst case 
% % We define the \emph{variation bound} of the derivative of the interference function $f$ as $2L_f \triangleq f^{'}_{\text{max}}-f^{'}_{\text{min}}$, then the optimal root locus can be expressed as
% % \begin{align} \label{eqn:osc}
% %   m_s &= -\frac{m_1}{2}  + \frac{\sqrt{m_1^2+4 L_f^2}}{2},\\
% %   a_{\text{min}} &= -a_{\text{max}} = 1 - \frac{2}{1 + \sqrt{1+\left(\frac{2L_f}{m_1}\right)^2} + \frac{2L_f}{m_1}}.
% % a^i_{1_{\text{min}}} &= 1 - \frac{2}{1 + \sqrt{1+\left(\frac{2L_f}{m_1}\right)^2} + \frac{2L_f}{m_1}} \le a^i_1 \le a^i_{1_{\text{max}}} = 1 - \frac{2}{1 + \sqrt{1+\left(\frac{2L_f}{m_1}\right)^2} -\frac{2L_f}{m_1}}.
% % \end{align}
% % The optimal value of $m_s$ which achieves  (\ref{eqn:osc}) is
% % \begin{align}
% %     m_s = -\frac{m_1}{2}  + \frac{\sqrt{m_1^2+4 L_f^2}}{2}.
% % \end{align}
% % If the interference function $f$ satisfies Definition \ref{def:inteference}, 
% % \begin{align} \label{eqn:optms_nonorm}
% %     m_s = \sqrt{\left(\frac{m_1}{2}\right)^2+A^2\omega^2} -\frac{m_1}{2} = \left(\sqrt{\left(\frac{1}{2}\right)^2+\left(\frac{A\omega}{m_1}\right)^2} -\frac{1}{2}\right)m_1.
% % \end{align}
% % By substituting (\ref{eqn:def_omega_star}), (\ref{eqn:def_a_star}) and (\ref{eqn:ms_norm}) into (\ref{eqn:optms_nonorm}),
% % \begin{align}
% %      m_s^* & = \sqrt{\frac{1}{4} + \left(2\pi \omega^{*}_{\text{int}}A^*_{\text{int}}\right)^2} - \frac{1}{2}.
% % \end{align}
% \subsection{Linearized Model of the Current-Control Loop with the General Linear Filter}
% By assuming the continuity condition, we linearize the model of current-control loop as:
% \begin{align}
%      \tilde{i}_c [n] = \, & q(T_{\text{on}})q(T_{\text{off}})\, \tilde{i}_c[n-1] +
%      q^{'}(t)\bigg\rvert_{t = T_{\text{on}}} q(T_{\text{off}}) I_c\, \tilde{t}_{\text{on}}[n] \nonumber \\
%      & + \left( u(t) * h(t)\right)\bigg\rvert_{t  = T_{\text{on}}}  \tilde{i}_p[n-1] \nonumber \\
%      & + (I_p-m_1T_{\text{off}})\left( u(t) * h(t)\right)^{'} \bigg\rvert_{t = T_{\text{on}}} \tilde{t}_{\text{on}} [n]
%      \nonumber \\
%      & + \left(m_1t\, u(t) * h(t)\right)^{'}\bigg\rvert_{t = T_{\text{on}}} \tilde{t}_{\text{on}} [n] \nonumber \\ 
%      & + \left(w(t)\, u(t) * h(t)\right)^{'}\bigg\rvert_{t = T_{\text{on}}} \tilde{t}_{\text{on}} [n]
% \end{align}
% % The zero state response of the low-pass filter given input signal $m_1t\,u(t)$ is
% % \begin{align}
% %      m_1t\, u(t)*h(t) = m_1\left(t + (e^{-\frac{t}{\tau}}-1)\tau \right) u(t)
% % \end{align}
% For all $t>0^{+}$, $u(t)*h(t)$ and $m_1t\,u(t)*h(t)$ are differentiable
% \begin{align}
%      \label{eqn:conv_eq1} \left( m_1t\, u(t)*h(t) \right)^{'} &=  m_1u(t)*h(t) \\
%      \label{eqn:conv_eq2} \left( u(t)*h(t) \right)^{'} &=  h(t)
% \end{align}
% By Substituting (\ref{eqn:conv_eq1}), (\ref{eqn:conv_eq2}), we have
% \begin{align} 
%     % \label{eqn:uhconv} u(t)*h(t) &= \left(1 -e^{-\frac{t}{\tau}}\right)u(t) = (1 - d)u(t), \\
%     % \label{eqn:sinapprox} A\,\omega\, \text{cos}(\omega  t+\varphi)\,u(t) * h(t) + A\,\text{sin}\,\varphi\, h(t) &=  \frac{A \,\omega \,\text{sin}(\omega t + \varphi + \delta)}{\sqrt{1+\omega^2\tau^2}} - \frac{A\, \omega \,\text{sin}( \varphi + \delta)}{\sqrt{1+\omega^2\tau^2}} e^{-\frac{t}{\tau}} + \frac{A\, \text{sin} \,\varphi}{\tau} e^{-\frac{t}{\tau}} \nonumber \\
%     %  & \approx \frac{A\, \text{sin}(\omega t + \varphi + \delta)}{\tau} - \frac{A\, \text{cos}( \varphi + \frac{\delta}{2})\, \text{sin} (\frac{\delta}{2})}{\tau}\, e^{-\frac{t}{\tau}}  \nonumber \\
%     %  &\approx \frac{A\,\text{sin}(\omega t + \varphi)}{\tau},
%      \tilde{i}_c [n] = & q(T_{\text{on}})q(T_{\text{off}})\, \tilde{i}_c[n-1] + \left( u(t) * h(t)\right)\bigg\rvert_{t  = T_{\text{on}}}  \tilde{i}_p[n] \nonumber \\
%      & + q^{'}(t)\bigg\rvert_{t = T_{\text{on}}} q(T_{\text{off}}) I_c\,\tilde{t}_{\text{on}}[n] \nonumber \\
%      & + (I_p-m_2T_{\text{off}}) h(T_{\text{on}}) \tilde{t}_{\text{on}} [n] \nonumber \\
%      & +\left(w(t)\, u(t) * h(t)\right)^{'}\bigg\rvert_{t= T_{\text{on}}} \tilde{t}_{\text{on}} [n]
% \end{align}
% We denote
% \begin{align}
%     c_1 = & \left( u(t) * h(t)\right)\bigg\rvert_{t  = T_{\text{on}}} \nonumber \\
%     c_2 = & q^{'}(t)\bigg\rvert_{t = T_{\text{on}}} q(T_{\text{off}}) I_c\,+(I_p-m_2T_{\text{off}}) h(T_{\text{on}}) \nonumber \\
%     & +\left(w(t)\, u(t) * h(t)\right)^{'}\bigg\rvert_{t= T_{\text{on}}} \nonumber \\
% \end{align}
% The resulting model is
% \begin{align}
%     \tilde i_p[n] = \; & \tilde i_p[n-1]  +m_1 \, \tilde t_{\text{on}}[n], \\
%     \tilde i_c [n] = \; & q(T_{\text{on}}) q(T_{\text{off}}) \,\tilde i_c [n-1] +  c_1 \, \tilde i_p [n] +  c_2 \, \tilde t_{\text{on}}[n].
% \end{align}
% \subsection{Linearized Model of the Current-Control Loop with First-Order Low Pass Filter}
% The zero state response of the first-order low-pass filter given input signal $u(t)$ is
% \begin{align} \label{eqn:u_conv_h}
%      u(t)*h(t) = \left( 1 - e^{-\frac{t}{\tau}}\right) u(t)
% \end{align}
% The zero state response of the first-order low-pass filter given input signal $m_1t\,u(t)$ is
% \begin{align} \label{eqn:tu_conv_h}
%      m_1t\, u(t)*h(t) = m_1\left(t + (e^{-\frac{t}{\tau}}-1)\tau \right) u(t)
% \end{align}
% % For all $t>0^{+}$, $m_1t\,u(t)*h(t)$ is differentiable
% % \begin{align}
% %      \label{eqn:conv_eq1}\left( m_1t\, u(t)*h(t) \right)^{'} &= m_1 \left (1-e^{-\frac{t}{\tau}} \right) u(t)
% % \end{align}
% By substituting (\ref{eqn:u_conv_h}) and (\ref{eqn:tu_conv_h}) into (\ref{eqn:equic}), the equilibrium can be expressed as
% \begin{align} \label{eqn:equic}
%     I_c = & \frac{\left(\left( I_p -m_2T_{\text{off}} + m_1 \, t + w(t) \right) u(t)*h(t)\right)\bigg\vert_{t=T_{\text{on}}}
%     }{1-q(T_{\text{on}})q(T_{\text{off}})} \nonumber \\
%     = & \, \frac{1-e^{-\frac{T_{\text{on}}}{\tau}}}{1-e^{-\frac{T}{\tau}}}(I_p - m_2T_{\text{off}}) + \left(1 + \frac{(e^{-\frac{T_{\text{on}}}{\tau}}-1)}{\frac{T_{\text{on}}}{\tau}} \right) m_1T_{\text{on}} \nonumber \\
%     & + \frac{g(T_{\text{on}}) - \frac{g(0)}{q(0)} q(T_{\text{on}})}{1-e^{-\frac{T}{\tau}}}
% \end{align}

% The resulting model is
% \begin{align} \label{eqn:filter_lin_sysx1}
% \tilde i_p[n] = \; & \tilde i_p[n-1]  +m_1 \, \tilde t_{\text{on}}[n], \nonumber \\
% \tilde i_c [n] = \; & b \,\tilde i_c [n-1] +  c_1 \, \tilde i_p [n] +  c_2 \, \tilde t_{\text{on}}[n],
% \end{align}
% where
% \begin{align}
%     c_1 & = 1 - d, \nonumber \\
%     c_2 & =  -\frac{b}{\tau}\,I_c + \frac{d}{\tau}\,I_v
%     + \frac{w(T_{\text{on}})}{\tau} + \frac{e^{-\frac{T_{\text{on}}}{\tau}}}{\tau}\int_{-\infty}^{+\infty} \frac{W(\omega)}{j\omega}\,d\omega\nonumber \\
%     b &=  e^{-\frac{T}{\tau}}  \nonumber \\
%     d &= e^{-T_{\text{on}}/\tau}.
% \end{align}
% \section{Proof of the Theorem \ref{theorem:taomin4stability}} \label{proof:taomin4stability}
% \begin{proof}
% We notice that the dynamics of the current controller is relevant with the peak inductor current $I_p$, namely the operating point. 
% From the block diagram, the closed-loop pole locates at 
% \begin{align} \label{eqn:cl_pole}
%      a  = 1 - \beta
% \end{align}
% where
% \begin{align} \label{eqn:cl_pole_param}
%   \beta & = \frac{m_1}{s},  \quad b = e^{-\frac{T}{\tau}}, \quad d = e^{-\frac{T_{\text{on}}}{\tau}}, \nonumber \\
%     s & = m_1 +  \frac{\psi_1 + \psi_2}{1-d}, \nonumber \\
%      \psi_1 & = \frac{w(T_{\text{on}})}{\tau} + \frac{e^{-\frac{T_{\text{on}}}{\tau}}}{\tau}\int_{-\infty}^{+\infty} \frac{W(\omega)}{j\omega}\,d\omega, \quad
%      \nonumber \\
%      \psi_2 & = - \frac{e^{-\frac{T}{\tau}}}{\tau}I_c + \frac{e^{-\frac{T_{\text{on}}}{\tau}}}{\tau}I_v.
% %    \label{eqn:transzparam}
% \end{align}
% The sufficient and necessary condition for stability is the closed-loop pole $a$ locates inside the unit disk. 
% \begin{proposition}
% Given any peak inductor current $I_p$, the $s$ is bounded from below by $s_1$, 
% \begin{align} \label{eqn:s_lower_bound1}
%     % = & m_1 + \frac{- \frac{\left[ m_1 t + A \, \text{sin}(\omega  t+\varphi) \right] u(t) * h(t)
%     % }{\left(1 - b\right)} \frac{b}{\tau} + \frac{A\, \text{sin}(\omega T_{\text{on}}+\varphi)}{\tau}}{1-d} \nonumber \\
%     s_1 = &  \left( m_1 - \frac{b \,t\,u(t)*h(t)}{(1-b)(1-d)\tau} m_1-\frac{b\,w(t) u(t)*h(t)}{(1-b)(1-d)\tau} \right) \bigg\vert_{t = T_{\text{on}}} \nonumber \\
%     & + \frac{1}{1-d} \left( \frac{w(t)}{\tau} + \frac{e^{-\frac{t}{\tau}}}{\tau}\int_{-\infty}^{+\infty} \frac{W(\omega)}{j\omega}\,d\omega \right) \bigg\vert_{t = T_{\text{on}}},
% \end{align}
% where $b = e^{-\frac{T}{\tau}}$ and  $d = e^{-\frac{T_{\text{on}}}{\tau}}$.
% $s_1$ is reached iff  $I_p = m_2 T_{\text{off}}$ (i.e. $I_v = 0$).
% \end{proposition}
% \begin{proof}
% We view $s$ as a function of $I_v$
% \begin{align}
%     s(I_v) = &  m_1 + \frac{d}{(1-d)\tau}I_v - \frac{b}{(1-d)\tau}I_c + \frac{1}{(1-d)\tau} w(T_{\text{on}}) \nonumber \\
%     & + \frac{d}{(1-d)\tau}\int_{-\infty}^{+\infty} \frac{W(\omega)}{j\omega}\,d\omega 
% \end{align}
% We view $I_c$ in as a function of $I_v$
% \begin{align}
%     I_c(I_v) = \frac{1}{1-b} I_v + C
% \end{align}
% where
% \begin{align}
%     C = \left(1 + \frac{(e^{-\frac{T_{\text{on}}}{\tau}}-1)}{\frac{T_{\text{on}}}{\tau}} \right) m_1T_{\text{on}} + \frac{g(T_{\text{on}}) - \frac{g(0)}{q(0)} q(T_{\text{on}})}{1-e^{-\frac{T}{\tau}}}.
% \end{align}
% Because $b = d\,e^{-\frac{T_{\text{off}}}{\tau}}<d$
% \begin{align}
%     \frac{\partial I_c}{\partial I_v} = \frac{1-d}{1-b} < 1,
% \end{align}
% Therefore
% \begin{align}
%     \frac{\partial s}{\partial I_v} = \frac{d}{\tau} - \frac{1-d}{1-b} \frac{b}{\tau} > \frac{d}{\tau} - \frac{b}{\tau} > 0.
% \end{align}
% $s$ is monotonically increasing function with respect to $I_v$. Therefore, the minimum $s$ is reached at $I_v = 0$. we proved (\ref{eqn:s_lower_bound1}).
% \end{proof}

% \begin{proposition}
% Given any interference with frequency $\omega\,\tau \ge 2\pi$, the $s_1$ is bounded from below by $s_2$,
% \begin{align} \label{eqn:s_lower_bound2}
%     s_2 = \left( 1- k_0 - \frac{A}{m_1 T_{\text{on}}} k_1 \right)m_1.
% \end{align}
% \end{proposition}

% \begin{proof}
% % \begin{align}
% %     a_1^i &= 1 - \frac{m_1(1-e^{-T_{\text{on}}/\tau})}{m_1(1-e^{-T_{\text{on}}/\tau}) - \left( \frac{m_1(T_{\text{on}}+\tau e^{-T_{\text{on}}/\tau}-\tau)+ \frac{A \, \text{sin}(\omega  T_{\text{on}} +\varphi)}{\omega \tau}}{\left(1-e^{-(T_\text{on}+T_{\text{off}})/\tau}\right)}\right) \frac{e^{-(T_{\text{on}} +T_{\text{off}}) /\tau}}{\tau} + \frac{A\, \text{cos}(\omega T_{\text{on}}+\varphi)}{\tau}}, \nonumber \\
% %     b^{i}_1 & =  e^{-T/\tau},  \nonumber \\
% %     \beta & = \frac{m_1}{m_1(1-e^{-T_{\text{on}}/\tau}) - \left( \frac{m_1(T_{\text{on}}+\tau e^{-T_{\text{on}}/\tau}-\tau)+ \frac{A \, \text{sin}(\omega  T_{\text{on}} +\varphi)}{\omega \tau}}{\left(1-e^{-(T_\text{on}+T_{\text{off}})/\tau}\right)}\right) \frac{e^{-(T_{\text{on}} +T_{\text{off}}) /\tau}}{\tau} + \frac{A\, \text{cos}(\omega T_{\text{on}}+\varphi)}{\tau}}. 
% % \end{align}
% We use the following approximations to simplify (\ref{eqn:s_lower_bound1})
% \begin{align} \label{eqn:s_lower_bound1_simp1}
%     t\;u(t)*h(t) = \left(t + (e^{-\frac{t}{\tau}}-1)\tau \right) u(t),
% \end{align}

% % \begin{align}  \label{eqn:s_lower_bound2}
% %     \cdots \approx m_1 - \frac{b(T_{\text{on}} + (d-1)\tau)}{(1-b)(1-d)\tau} m_1 + \frac{A\text{sin}(\omega T_{\text{on}}+\varphi)}{(1-d)\tau}
% % \end{align}
% Substitute (\ref{eqn:s_lower_bound1_simp1}) to (\ref{eqn:s_lower_bound1})
% \begin{align} \label{eqn:s_lower_bound1_bound2}
%     s_1  = & m_1  - \frac{b}{(1-b)(1-d)\tau} \left( 1 + \frac{d-1}{T_{\text{on}}/\tau}\right)  m_1T_{\text{on}}  \nonumber \\
%     & - \frac{b}{(1-b)(1-d)\tau}\left(g(T_{\text{on}}) - dg(0)\right)
%     \nonumber \\
%     & + \frac{1}{(1-d)\tau}\left( f( T_{\text{on}}) + d\,g(0) \right) \nonumber
% \end{align}
% % Substitute (\ref{eqn:s_lower_bound1_simp2}) into (\ref{eqn:s_lower_bound2})
% \begin{align}
%      s_1 \ge \, & m_1 -
%     \frac{ m_1T_{\text{on}} b }{(1-b)(1-d)\tau} \left( 1 + \frac{d-1}{T_{\text{on}}/\tau}\right) \nonumber\\
%     & - \frac{b}{(1-b)(1-d)\tau}(1+d)\frac{A}{\omega \tau} \nonumber\\
%     & - \frac{1}{(1-d)\tau} \frac{A}{\omega \tau} - \frac{1}{(1-d)\tau} A \nonumber \\
%     \approx & \, \left(1- k_0 - \frac{A}{m_1 T_{\text{on}}} k_1 \right)m_1,
% \end{align}
% where
% \begin{align}
%     k_0 & = \frac{b(1 + \tau^* d -\tau^*)}{(1-b)(1-d)\tau^*}, \quad k_1 = \frac{1}{\tau^*(1-d)}, \nonumber \\
%     b & = e^{-\frac{T}{\tau}}, \quad d = e^{-\frac{T_{\text{on}}}{\tau}}, \quad \tau^* = \frac{\tau}{T_{\text{on}}}, \quad A^* = \frac{A}{m_1T_{\text{on}}} \nonumber .
% \end{align}
% We proved (\ref{eqn:s_lower_bound2}).
% \end{proof}
% % The approximation from (\ref{eqn:s1algebra_1}) to (\ref{eqn:s1algebra_2}) is justified by proving
% % \begin{align}
% %     m_1T_{\text{on}} \left( 1 + \frac{d-1}{T_{\text{on}}/\tau}\right) \gg \frac{Ad\,\text{cos}\varphi}{\omega \tau}.
% % \end{align}
% % \begin{proof}
% % We define an auxiliary function
% % \begin{align}
% %     & y(x) \triangleq  e^{\frac{1}{x}} + x \left(1-e^{\frac{1}{x}}\right),\\
% %     & y(1)= 1, \quad y(1.5) = 0.53.
% % \end{align}
% % Therefore, if we assume $\tau \le 1.5\, T_{\text{on}}$ and $A \le m_1 T_{\text{on}}$,
% % \begin{align} \label{eqn:uplimitonc}
% %     \frac{m_1T_{\text{on}} \left( 1 + \frac{d-1}{T_{\text{on}}/\tau}\right)}{\frac{Ad\,\text{cos}\varphi}{\omega \tau}} & = \frac{m_1T_{\text{on}}}{A\,\text{cos}\varphi} y\left(\frac{\tau}{T_{\text{on}}} \right) \omega \tau \nonumber\\
% %     & \ge \frac{\omega \tau}{2} \gg \frac{\omega \tau}{2 \pi} \ge 1.
% % \end{align}
% % \end{proof}

% % The stability of inner current loop should be guaranteed for any input noise phase $\varphi$, hence (\ref{eqn:s_lower_bound1}) can be further extended as
% % \begin{align}  \label{eqn:s_lower_bound2}
% %     \cdots \ge (1- k_0 - \frac{A}{\omega} k_1 - A k_2)m_1   
% % \end{align}
% % where 
% % \begin{align}
% %      k_0 = \frac{d tu(t)*h(t)}{(1-c)(1-d)\tau} \bigg\rvert_{t = T_{\text{on}}} \quad k_1 = \frac{d(1+d)}{m_1(1-c)(1-d)\tau^2} \quad k_2 = \frac{1}{m_1(1-d)\tau}. 
% % \end{align}


% % For ease of calculation, we denote 
% % \begin{align}
% %      k(\tau, \omega; \varphi) =  \left( \frac{ \frac{\text{sin}(\omega T_{\text{on}} +\varphi)}{\omega^2 \tau}}{\left(1-e^{-(T_\text{on}+T_{\text{off}})/\tau}\right)}\right) \frac{e^{-(T_{\text{on}} +T_{\text{off}}) /\tau}}{\tau m_1} - \frac{ \text{cos}(\omega T_{\text{on}}+\varphi)}{\omega \tau }\\
% %      l(\tau) =  \left( \frac{(T_{\text{on}}+\tau e^{-T_{\text{on}}/\tau}-\tau)}{\left(1-e^{-(T_\text{on}+T_{\text{off}})/\tau}\right)}\right) \frac{e^{-(T_{\text{on}} +T_{\text{off}}) /\tau}}{\tau m_1}
% % \end{align}
% % From (\ref{eqn:s_lower_bound2}), the pole of (\ref{eqn:filter_ztransform}) is lowered bounded by
% % \begin{align}
% %     a \ge  1 - \frac{1}{1 - (k_0 + \frac{A}{\omega} k_1  + A k_2 )}
% % \end{align}

% % From the theorem, we have the stability condition is. Therefore, if the filter $\tau$ satisfies the following equations, the stability of inner current loop is guaranteed: 
% % \begin{align}
% %     k_0 + \frac{A_{\text{min}}}{\omega_{\text{max}}} k_1  + A_{\text{min}} k_2 < \frac{1}{2}
% % \end{align}
% Finally, we finish the proof of Theorem \ref{theorem:taomin4stability}.
% From (\ref{eqn:s_lower_bound2}), the closed-loop pole is bounded from below by
% \begin{align}
%     a \ge  1 - \frac{1}{1 - \left(k_0 + \frac{A}{m_1 T_{\text{on}}} k_1 \right)}.
% \end{align}
% Therefore, the stability of inner current loop is guaranteed if the filter $\tau$ satisfies
% \begin{align}
%     k_0 + \frac{A}{m_1 T_{\text{on}}} k_1 < \frac{1}{2}.
% \end{align}
% \end{proof}


% \end{appendices}
